# Supplementary material for: Experimental observation of a topological band gap opening in ultracold Fermi gases with two-dimensional spin-orbit coupling
Source: arXiv:1511.08492 source file (2016-12-03)
Supplement: Supplementary file 1 [file SI-PRL-11-09.pdf]

# Supplementary Information for "Experimental observation of topological band gap opening in ultracold Fermi gases with two-dimensional spin-orbit coupling"

Zengming Meng,[1,2] Lianghui Huang,[1,2] Peng Peng,[1] Donghao Li,[1] Liangchao Chen,[1] Yong Xu,[3] Chuanwei Zhang,[3] Pengjun Wang,[1,2] and Jing Zhang[†1,4]

[1]*State Key Laboratory of Quantum Optics and Quantum Optics Devices, Institute of Opto-Electronics, Shanxi University, Taiyuan 030006, P.R.China*
[2]*Collaborative Innovation Center of Extreme Optics, Shanxi University, Taiyuan 030006, P.R.China*
[3]*Department of Physics, The University of Texas at Dallas, Richardson, Texas 75080-3021, USA*
[4]*Synergetic Innovation Center of Quantum Information and Quantum Physics, University of Science and Technology of China, Hefei, Anhui 230026, P. R. China*

## I. EFFECTIVE SPIN-HALF HAMILTONIAN

Here we derive the effective $2 \times 2$ spin Hamiltonian (Eq. (2) in the main text) from the full $3 \times 3$ Hamiltonian (Eq. (1) in the main text).

We write the Hamiltonian in Eq. (1) in the main text as the dimensionless one with the energy unit $E_r$ and the momentum unit $k_r$,

$$\tilde{H}_{xy} = \begin{pmatrix} (\mathbf{p}-\mathbf{k}_1)^2 & -\frac{\bar{\Omega}^i_{12}}{2} - i\frac{\Gamma^i_{12}}{2} & -\frac{\Omega^i_{13}}{2} \\ -\frac{\bar{\Omega}^i_{12}}{2} + i\frac{\Gamma_{12}}{2} & (\mathbf{p}-\mathbf{k}_2)^2 + \delta_2 & -\frac{\Omega^i_{23}}{2} \\ -\frac{\Omega^i_{13}}{2} & -\frac{\Omega^i_{23}}{2} & (\mathbf{p}-\mathbf{k}_3)^2 + \delta_3 \end{pmatrix}. \tag{S1}$$

where $i = I$ or $II$ for case I or II. $\bar{\Omega}^i_{12}$ and $\Gamma^i_{12}$ are the real and imaginary parts of $\Omega^i_{12}$. $\bar{\Omega}^I_{12} = \Omega_{12}$, $\bar{\Omega}^{II}_{12} = \Omega_{12}\cos^2\theta$, $\Gamma^I_{12} = 0$, $\Gamma^{II}_{12} = \Omega_{12}\sin^2\theta$. Other parameters are the same as that in the main text. To obtain the degenerate dark states in the adiabatic approximation, we transfer the Hamiltonian back to the original position-dependent space

$$\tilde{H}_{xy} = \mathbf{p}^2 + \tilde{H}_1 + \tilde{H}_2 + \tilde{H}_Z, \tag{S2}$$

where

$$\tilde{H}_1 = \begin{pmatrix} -\bar{\Omega}^i_{12}\Omega^i_{13}/(2\Omega^i_{23}) & -\frac{\bar{\Omega}^i_{12}}{2}e^{-2iy} & -\frac{\Omega^i_{13}}{2}e^{i(x-y)} \\ -\frac{\bar{\Omega}^i_{12}}{2}e^{2iy} & -\bar{\Omega}^i_{12}\Omega^i_{23}/(2\Omega^i_{13}) & -\frac{\Omega^i_{23}}{2}e^{i(x+y)} \\ -\frac{\Omega^i_{13}}{2}e^{i(-x+y)} & -\frac{\Omega^i_{23}}{2}e^{-i(x+y)} & -\Omega^i_{13}\Omega^i_{23}/(2\bar{\Omega}^i_{12}) \end{pmatrix}, \tag{S3}$$

$$\tilde{H}_2 = \bar{\Omega}^i_{12}\Omega^i_{13}/(2\Omega^i_{23}) + \begin{pmatrix} 0 & 0 & 0 \\ 0 & \delta^i_2 & 0 \\ 0 & 0 & \delta^i_3 \end{pmatrix}, \tag{S4}$$

$$\tilde{H}_Z = \begin{pmatrix} 0 & -i\frac{\Gamma^i_{12}}{2}e^{-2iy} & 0 \\ i\frac{\Gamma^i_{12}}{2}e^{2iy} & 0 & 0 \\ 0 & 0 & 0 \end{pmatrix}, \tag{S5}$$

with $\delta^i_2 = -\left[\bar{\Omega}^i_{12}\Omega^i_{13}/(2\Omega^i_{23}) - \bar{\Omega}^i_{12}\Omega^i_{23}/(2\Omega^i_{13})\right] + \delta_2$ and $\delta^i_3 = -\left[\bar{\Omega}^i_{12}\Omega^i_{13}/(2\Omega^i_{23}) - \Omega^i_{13}\Omega^i_{23}/(2\bar{\Omega}^i_{12})\right] + \delta_3$.

The eigenstates of atom-light interaction Hamiltonian $\tilde{H}_1$ contain two degenerate dark states $|D_1\rangle$ and $|D_2\rangle$ with the energy $E_{D_1} = E_{D_2} = 0$ and one bright state with $E_B = -\frac{1}{2}\left(\frac{\bar{\Omega}^i_{12}\Omega^i_{13}}{\Omega^i_{23}} + \frac{\bar{\Omega}^i_{12}\Omega^i_{23}}{\Omega^i_{13}} + \frac{\Omega^i_{23}\Omega^i_{13}}{\bar{\Omega}^i_{12}}\right)$. The two degenerate dark states are

$$|D^i_1\rangle = N^i_1\left(-\Omega^i_{23}e^{-iy}|1\rangle + \Omega^i_{13}e^{iy}|2\rangle\right), \tag{S6}$$

$$|D^i_2\rangle = N^i_2\left(\Omega^i_{13}e^{-iy}|1\rangle + \Omega^i_{23}e^{iy}|2\rangle - \Omega^i_3 e^{-ix}|3\rangle\right), \tag{S7}$$

where $\Omega^i_3 = \bar{\Omega}^i_{12}\frac{\Omega^{i2}_{13}+\Omega^{i2}_{23}}{\Omega^i_{13}\Omega^i_{23}}$, $N^i_1 = \frac{1}{\sqrt{\Omega^{i2}_{23}+\Omega^{i2}_{13}}}$, and $N^i_2 = \frac{1}{\sqrt{\Omega^{i2}_{13}+\Omega^{i2}_{23}+\Omega^{i2}_{3}}}$. In the experiment, $\bar{\Omega}^i_{12} < 0$ and $\Omega^i_{13}, \Omega^i_{23} > 0$, therefore $E_B > 0$ and two dark states are the ground states.

We assume that the quantum state of an atom adiabatically stays in the subspace spanned by the two degenerate dark states, thus the state can be written as $|\psi\rangle = \psi_1^i(\mathbf{r},t)|D_1^i\rangle + \psi_2^i(\mathbf{r},t)|D_2^i\rangle$. $\psi(\mathbf{r},t) = [\psi_1^i(\mathbf{r},t), \psi_2^i(\mathbf{r},t)]^T$ satisfies the following equation

$$i\partial_t\psi(\mathbf{r},t) = H_{eff}\psi(\mathbf{r},t), \tag{S8}$$

with the effective $2\times 2$ Hamiltonian

$$H_{eff} = \mathbf{p}^2 + \gamma_y^i p_y + \beta_x^i p_x + (-\alpha_y^i p_y + h_x^i)\sigma_x + \left[\beta_y^i p_y - \beta_x^i p_x + h_z^i\right]\sigma_z + h_\perp^i\sigma_y + \epsilon_0^i.$$

Here $\gamma_y^i = (\Omega_{23}^{i2} - \Omega_{13}^{i2})(N_1^{i2} - N_2^{i2})$, $\beta_x^i = N_2^{i2}\Omega_3^{i2}$, $\alpha_y^i = 4N_1^iN_2^i\Omega_{13}^i\Omega_{23}^i$, $h_x^i = N_1^iN_2^i\Omega_{13}^i\Omega_{23}^i\delta_2^i$, $\beta_y^i = (\Omega_{23}^{i2} - \Omega_{13}^{i2})(N_1^{i2} + N_2^{i2})$, $h_z^i = \left[(N_1^{i2}\Omega_{13}^{i2} - N_2^{i2}\Omega_{23}^{i2})\delta_2^i - N_2^{i2}\Omega_3^{i2}\delta_3^i\right]/2$, $h_\perp^i = -\frac{\Gamma_{12}^i}{2}N_1^iN_2^i(\Omega_{23}^{i2} + \Omega_{13}^{i2}) = -\frac{\Gamma_{12}^i}{2}N_2^i/N_1^i$, $h_0^i = \left[(N_1^{i2}\Omega_{13}^{i2} + N_2^{i2}\Omega_{23}^{i2})\delta_2^i + N_2^{i2}\Omega_3^{i2}\delta_3^i\right]/2$, and $\epsilon_0^i = \bar{\Omega}_{12}^i\Omega_{13}^i/(2\Omega_{23}^i) + h_0^i + 1$.

For case I, $\Gamma_{12}^I = 0$, thus $h_\perp^I = 0$. In this case, the Dirac cone appears at $p_y = h_x^i/\alpha_y^i = \delta_2^i/4$ and $p_x = (h_z^i + \beta_y^i h_x^i/\alpha_y^i)/\beta_x^i = (h_z^i + \beta_y^i\delta_2^i/4)/\beta_x^i$. In case II, $\Gamma_{12}^{II} \neq 0$ and $h_\perp^{II} \neq 0$, a band gap is opened at the Dirac point.

Using the transformation

$$\begin{pmatrix}\psi_1^i\\ \psi_2^i\end{pmatrix} = e^{i(-\gamma_y^i y - \beta_x^i x)/2}e^{-i\pi/4\sigma_x}\begin{pmatrix}\phi_1^i\\ \phi_2^i\end{pmatrix},$$

the effective Hamiltonian (the Eq. (2) in the main text) can be written as

$$H_{eff} = \mathbf{p}^2 + H_{SOC}^i + V_I^i + V_z^i\sigma_z + \tilde{\epsilon}_0^i, \tag{S9}$$

where the 2D SOC $H_{SOC}^i = -\alpha_y^i p_y\sigma_x + \left(\beta_x^i p_x - \beta_y^i p_y\right)\sigma_y$, the in-plane Zeeman field $V_I^i = V_x^i\sigma_x + V_y^i\sigma_y$ with $V_x^i = \alpha_y^i\gamma_y^i/2 + h_x^i$ and $V_y^i = \beta_x^{i2}/2 + \beta_y^i\gamma_y^i/2 - h_z^i$, the perpendicular Zeeman field $V_z^i = h_\perp^i$, and the constant energy shift $\tilde{\epsilon}_0^i = \epsilon_0^i - \beta_x^{i2}/4 - \gamma_y^{i2}/4$. For the specific case that $-\Omega_{12}^i = \Omega_{23}^i = \Omega_{13}^i = \Omega$, $\delta_2 = \delta_3 = 0$, we have $N_1^i = \frac{1}{\sqrt{2\Omega}}$, $N_2^i = \frac{1}{\sqrt{6\Omega}}$, $\alpha_x^i = \frac{2}{\sqrt{3}}$, $\beta_x^i = \frac{2}{3}$, and $h_x^i = h_0^i = h_z^i = \gamma_y^i = \beta_y^i = 0$. The effective Hamiltonian reduces to

$$H_{eff} = \mathbf{p}^2 - \frac{2}{\sqrt{3}}p_y\sigma_x + \frac{2}{3}p_x\sigma_y + \frac{2}{9}\sigma_y + V_z\sigma_z \tag{S10}$$

In case I, $\bar{\Omega}_{12}^I = \Omega_{12}$, $\Omega_{13}^I = \Omega_{13}\cos\theta$, $\Omega_{23}^I = \Omega_{23}\cos\theta$, and $\Gamma_{12}^I = 0$, and there exist a Dirac point. In case II, $\bar{\Omega}_{12}^{II} = \Omega_{12}\cos^2\theta$, $\Omega_{13}^{II} = \Omega_{13}\cos\theta$, $\Omega_{23}^{II} = \Omega_{23}\cos\theta$, and $\Gamma_{12}^{II} = \Omega_{12}\sin^2\theta$, a band gap

$$\Delta = 2|V_z^{II}| = \sin^2\theta\left[\Omega_{12}^{-2} + \cos^2\theta\left(\Omega_{13}^{-2} + \Omega_{23}^{-2}\right)\right]^{-1/2}. \tag{S11}$$

is opened at the Dirac point

$$\begin{aligned} p_y^{II} &= \frac{\Omega_{12}}{8}\frac{\Omega_{23}^2 - \Omega_{13}^2}{\Omega_{13}\Omega_{23}}\cos^2\theta + \frac{\delta_2}{4} \\ p_x^{II} &= (h_z^{II} + \beta_y^{II}p_y^{II})/\beta_x^{II}. \end{aligned} \tag{S12}$$

## II. REALIZATION OF A PERPENDICULAR ZEEMAN FIELD

Here we provide detailed analysis on how to implement an effective perpendicular Zeeman field by generating an imaginary part of the Raman coupling strength $\Omega_{12}$ through simply manipulating the polarization of three Raman lasers. In the experiment, the Raman laser 3 couples the ground state $|3\rangle$ and propagates along the $x$ axis, whose polarization is fixed and linearly polarized along the $y$ direction $\overrightarrow{E}_3 = A_3\hat{\mathbf{e}}_\perp$, corresponding to the $\sigma$ polarization (relative to the quantization axis $\mathbf{z}$ defined by the magnetic field). The Raman laser 2 couples the ground state $|2\rangle$ and propagates along the $y$ axis. The linear polarization of the Raman laser 2 is initially prepared along the $x$ direction ($\sigma$ polarization) and rotated on the $xz$ plane by a $\lambda/2$ waveplate, yielding $\overrightarrow{E}_2 = A_2(\cos\theta\hat{\mathbf{e}}_\perp + \sin\theta\hat{\mathbf{e}}_\parallel)$, where $\hat{\mathbf{e}}_\perp$ and $\hat{\mathbf{e}}_\parallel$ components correspond to $\sigma$ and $\pi$ polarizations. The Raman laser 1 couples the ground state $|1\rangle$ and propagates along the $y$ axis. The linear polarization of the Raman laser 1 is prepared along the $z$ direction ($\pi$ polarization) and also rotated by an angle $\theta$ using a $\lambda/2$ waveplate ($\overrightarrow{E}_1 = A_1(\cos\theta\hat{\mathbf{e}}_\parallel + \sin\theta\hat{\mathbf{e}}_\perp)$) to keep orthogonal with the polarization of the Raman laser 2.

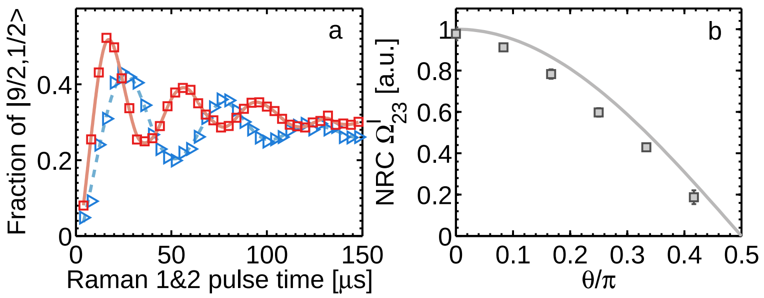


FIG. S1: Measure the Raman coupling strength by Rabi oscillations between two hyperfine ground states. (**a**) The population in $|2\rangle$ as a function of duration time of the Raman lasers 1 and 2 pulse. The red squares and blue triangles correspond to the polarization rotation angles $\theta = 0^o$ and $45^o$ respectively. The solid and dashed lines are fitting curves. (**b)** Plot of the Raman coupling strengths $\Omega^I_{23}$ versus $\theta$. The grey squares are from experiment and the solid line is from the theoretical $\cos\theta$ curve. NRC represents normalized Raman coupling.

The linear polarization of the Raman laser 1 can be further tuned to elliptical polarization by inserting a $\lambda/4$ waveplate with the optical axis aligned along the $\mathbf{z}$ direction after the $\lambda/2$ waveplate. Therefore we can consider two different cases for the polarization of the Raman laser 1 for comparison: I) linear polarization without the $\lambda/4$ waveplate; II) elliptical polarization with the $\lambda/4$ waveplate.

**Case I**: Because the difference $\Delta m = 0$ between the hyperfine Zeeman states $|2\rangle$ and $|3\rangle$, only $\sigma$-$\sigma$ polarization can drive the Raman transition between $|2\rangle$ and $|3\rangle$, yielding the Raman coupling strength $\Omega^I_{23} = \cos\theta A_2 A_3 r_{23} = \cos\theta\Omega_{23}$. Similarly, the difference $\Delta m = 1$ between states $|1\rangle$ and $|3\rangle$ allows only $\pi$-$\sigma$ polarization driven transition, yielding $\Omega^I_{13} = \cos\theta A_1 A_3 r_{13} = \cos\theta\Omega_{13}$. While $\Omega^I_{12} = A_1 A_2 r_{12}(\cos^2\theta + \sin^2\theta) = \Omega_{12}$ ($\Delta m = 1$ between states $|1\rangle$ and $|2\rangle$), which is unchanged when the linear polarizations of two Raman lasers keep orthogonal. We see such rotations keep the Hamiltonian (1) real, similar as that without the $\lambda/2$ waveplate (i.e., $\theta = 0$), therefore only shift the Dirac point position and cannot open a band gap.

**Case II:** The $\lambda/4$ waveplate inserted after the $\lambda/2$ waveplate for the Raman laser 1 changes the linear polarization to the elliptical polarization with $\overrightarrow{E}_1 = A_1(\cos\theta\hat{\mathbf{e}}_\parallel + i\sin\theta\hat{\mathbf{e}}_\perp)$. The resulting Raman coupling strengths $\Omega^{II}_{13} = \cos\theta\Omega_{13}$ and $\Omega^{II}_{23} = \cos\theta\Omega_{23}$ are the same as the case I because of the same parallel polarization component. While $\Omega^{II}_{12} = A_1 A_2 r_{12}(\cos^2\theta + i\sin^2\theta) = \Omega_{12}(\cos^2\theta + i\sin^2\theta)$, yielding an imaginary part $H_Z = -i\frac{\Omega_{12}\sin^2\theta}{2}|1\rangle\langle 2| + H.c$ in the Hamiltonian (1) in the main text.

The effective Raman coupling $\Omega^i_{jj'}$ for two cases after applying the waveplates can be measured using the Rabi

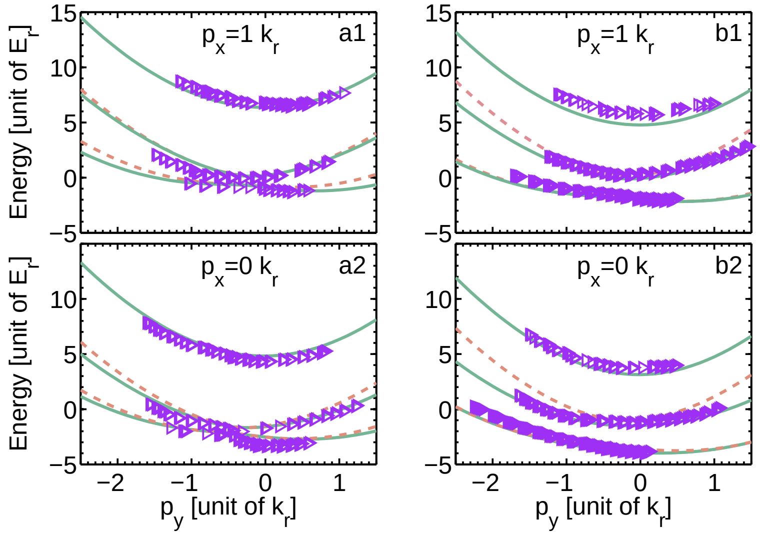


FIG. S2: Additional cross-section drawings of the energy dispersion in Fig. 2 in the main text in the energy-$p_y$ coordinates for different quasimomentum $p_x$. Triangles are from experimental data. Solid and dashed lines are from theoretical calculations using the full (Eq. 1) and effective (Eq. 2) Hamiltonians in the main text, respectively.

oscillation between two hyperfine ground states. For the measurement of $\Omega_{12}^{i}$ ($i = I$ or $II$), all atoms are initially prepared in the $|1\rangle$ state. The two-photon Raman detuning between Raman lasers 1 and 2 is set as $\delta_2 = -(\mathbf{k}_1 - \mathbf{k}_2)^2/2m$ so that the $p_y = 0$ momentum component of state $|1\rangle$ is at resonance with the $p_y = 2k_r$ component of state $|2\rangle$. We then apply a Raman pulse (without the Raman laser 3) to the system and measure the spin population for different duration times of the Raman pulse. We determine the value of the Raman coupling strength by fitting the measurement of the Rabi oscillation, as shown in Fig. S1(a). In Fig. S1(b), we show the dependence of $\Omega_{23}^{I}$ on the rotation angle $\theta$, which agrees with theoretical $\cos\theta$ curve as expected.

## III. EXPERIMENTAL SETUP AND PROCEDURE

Consider ultracold $^{40}$K Fermi gases with three relevant hyperfine states within the $4^2S_{1/2}$ ground electronic manifold, $|1\rangle = |F = 9/2, m_F = 3/2\rangle$, $|2\rangle = |F = 9/2, m_F = 1/2\rangle$, and $|3\rangle = |F = 7/2, m_F = 1/2\rangle$, where ($F$, $m_F$) are the quantum numbers for hyperfine ground states as shown in Fig. 1a in the main text. A homogeneous bias magnetic field $B_0 = 121.4$ G along the $z$ axis (the gravity direction) produces a Zeeman shift to isolate these three hyperfine states from others in the Raman transitions. We can neglect other hyperfine states and treat this system as one with three ground states. Three far-detuned Raman lasers propagating on the $xy$ plane couple these three ground states to the electronically excited states, which include a fine-structure doublet $4^2P_{1/2}$ ($D_1$ line) and $4^2P_{3/2}$ ($D_2$ line) with additional hyperfine structures.

In the experiment, we first precool the mixture of $^{87}$Rb atoms ($\sim 1\times 10^7$) at the spin state $|F = 2, m_F = 2\rangle$ and $^{40}$K atoms ($\sim 4\times 10^6$) at the spin state $|F = 9/2, m_F = 9/2\rangle$ to 1.5 $\mu K$ by radio-frequency evaporation cooling in the quadrupole-Ioffe configuration trap, and then transport them into the center of the glass cell in favor of optical access. Both species are loaded into the optical dipole trap, which consists with two far-resonance laser beams, at a wavelength of 1064 $nm$, crossing in the horizontal plane($\hat{x}\pm\hat{y}$). The degenerate Fermi gas of ($\sim 2\times 10^6$) $^{40}$K atoms in the lowest hyperfine Zeeman state $|F = 9/2, m_F = 9/2\rangle$ state is obtained by gradually decreasing the depth of the optical trap. The temperature of the Fermi gas is $0.2 \sim 0.3T_F$, where the Fermi temperature is defined by $T_F = \hbar\bar{\omega}(6N)^{1/3}/k_B$. Here $\bar{\omega} = (\omega_x\omega_y\omega_z)^{1/3}$ is the geometric mean of the optical trap frequency, $N$ is the particle number of $^{40}$K atoms, and $k_B$ is the Boltzmann's constant. For the $^{40}$K degenerate Fermi gas, the optical trap frequency is about $2\pi\times(80, 80, 80)$ Hz along ($\hat{x}$,$\hat{y}$,$\hat{z}$). We use a resonant laser beam pulse (780 $nm$) for 0.03 $ms$ to remove the $^{87}$Rb atoms in the mixture without losing and heating $^{40}$K atoms. Subsequently, the atoms of $|F = 9/2, m_F = 9/2\rangle$ state are transferred into the state $|9/2, 5/2\rangle$ via a rapid adiabatic passage induced by a rf field of 80 ms at 19.6 G. Here, the transition is driven by a rf ramp that starts from 6.56 MHz to the end of 6.28 MHz. Then a homogeneous bias magnetic field along the $z$ axis (gravity direction) is ramped to $B_0 = 121.4$ G by a pair of coils operating in the Helmholtz configuration.

Three Raman lasers are derived from a continuous-wave Ti-sapphire single frequency laser (M Squared lasers, SolsTiS). Two Raman beams 1 and 2 are frequency-shifted with the frequency difference about 38.8 MHz by two double-pass acousto-optic modulators (AOM), respectively. The Raman laser 3 is sent through two AOMs with double-pass and the frequency shifted about 1293 MHz (compared with the Raman laser 2). Then three Raman beams are coupled into three polarization maintaining single-mode fibers respectively in order to improve stability of the beam pointing and achieve better beam-profile quality. Behind the fibers, these three Raman beams have the maximum power 80 mW for each beam and they overlap in the atomic cloud with $1/e^2$ radii of 200 $\mu m$. The Raman lasers 1 and 2 counter-propagate along the y axis and the Raman laser 3 propagates along the x axis.

In the experiments, we take time-of-flight (TOF) absorption images after the rf field is applied at different frequencies. The transitions driven by rf field require the energy and momentum conservation with the relation between the energy of the $i$-th dressed state and that of the free reservoir state,

$$E_i(\mathbf{p}) = E_0(\mathbf{p}) - \hbar\nu_{rf} + E_z,$$

where $E_i(\mathbf{p})$ is the energy of the $i$-th band of the spin-orbit coupled Hamiltonian, $E_0(\mathbf{p}) = \mathbf{p}^2/2m$ is the dispersion of the initial reservoir state $|9/2, 5/2\rangle$, $\nu_{rf}$ is the frequency of the rf field, and $E_z$ is the Zeeman energy difference between $|9/2, 5/2\rangle$ and $|9/2, 3/2\rangle$. For the ideal case, the solution of this equation is a curve $C = \{\mathbf{p}^*\}$ with an infinitesimal width in the momentum space. Its length is determined by $k_F$ of the initial reservoir state. In reality, the finite width of the rf pulse leads to a finite resolution in the energy space. Thus, the curve representing the solution of equation (**??**) acquires a finite width. We use a Gaussian shape pulse of the rf field with 450 $\mu s$ to optimize the resolution in rf spectroscopy. In the TOF image, the full momentum width at half maximum of the atomic density is about $0.4 - 0.7k_r$ at the final state $|9/2, 3/2\rangle$ of rf spectroscopy. To extract $\mathbf{p}^*$, we use a Gaussian fit to locate the maximum of the measured atomic density. For a given rf frequency, the curve $C = \{\mathbf{p}^*\}$ is obtained. Using $\mathbf{p}^*$, we obtain the energy of the $i$-th dressed band $E_i(\mathbf{p}^*) = E_0(\mathbf{p}^*) - \hbar\nu_{rf} + E_z$.

Since $\mathbf{p}^*$ is a function of $\nu_{rf}$, we vary the rf frequency, obtain $\mathbf{p}^*$ and the resultant $E_i(\mathbf{p}^*)$ for each given rf frequency. This allows one to obtain a three-dimensional plot as shown in Fig. 2 (**a2**) and (**b2**) of the main text. It is worth

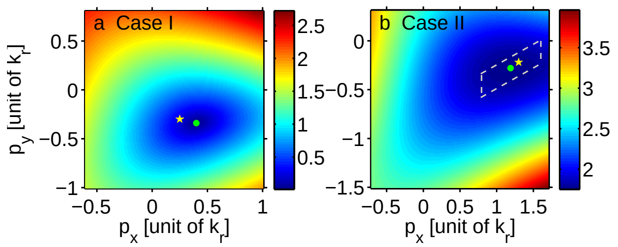


FIG. S3: (**a**,**b**) Plot of the energy differences between the lowest two bands in theory, calculated from the 3×3 Hamiltonian (1) in the main text. The stars and dots correspond to the Dirac point positions in experiments and theory, respectively. The parameters used are the same as that in Fig. 2 in the main text.

pointing out that, there are several reasons to make the measurements of single particle band structure not exactly agreeing with the calculations. The main practical issue in experiments is the stability of the magnetic field. To obtain the band structure, we need to repeat the experimental measurements at the different rf frequencies. Thus the stability of the magnetic field (especially the long term stability) will influence the measured rf spectrum. Due to the finite momentum width, the fitting process will also contribute to the quantitative disagreement. These issues led to the uncertainty of the energy and momentum in the dispersion curves.

In Fig. S2, we show some additional cross-section drawings of Fig. 2 (**a1**, **a2, b1, b2**) in the energy-$p_y$ coordinates for different $p_x$, which are away from the Dirac points. The experimental measured energy differences between the lowest two bands can be compared with the theoretical calculations obtained from the $3 \times 3$ Hamiltonian (1) (shown in Fig. S3), which shows good agreement.

## IV. BERRY CURVATURES

The topological properties of the induced band gap by the perpendicular Zeeman field can be described by the Berry curvature of each band $\mathcal{F}_{n\mathbf{p}} = \nabla_{\mathbf{p}} \times \mathbf{A}_{np}$ with the Berry connection $\mathbf{A}_{np} = i \langle u_{n\mathbf{p}} | \nabla_{\mathbf{p}} | u_{np} \rangle$, where $|u_{n\mathbf{p}}\rangle$ is the eigenstate of the Hamiltonian (1) in the main text. In case I, because all components of the Hamiltonian are real, the eigenstates $|u_{n\mathbf{p}}\rangle$ are real except at the degenerate Dirac point. Therefore $\mathbf{A}_{n\mathbf{p}} = \frac{1}{2} \nabla_{\mathbf{p}} \langle u_{n\mathbf{p}} | |u_{n\mathbf{p}}\rangle = 0$ except at the Dirac point, and the Berry curvature is a delta function at the Dirac point, similar as that in graphene. In case II, the imaginary part $H_Z$ makes the eigenstates $|u_{n\mathbf{p}}\rangle$ complex, and the Berry curvatures become nonzero for all $\mathbf{p}$ with a peak located at the Dirac point (see Fig. S4). The Berry phases $\Upsilon = \int d^2\mathbf{p}\mathcal{F}_{n\mathbf{p}}$ are found to be $\mp\pi$ for the lowest two bands, as expected.

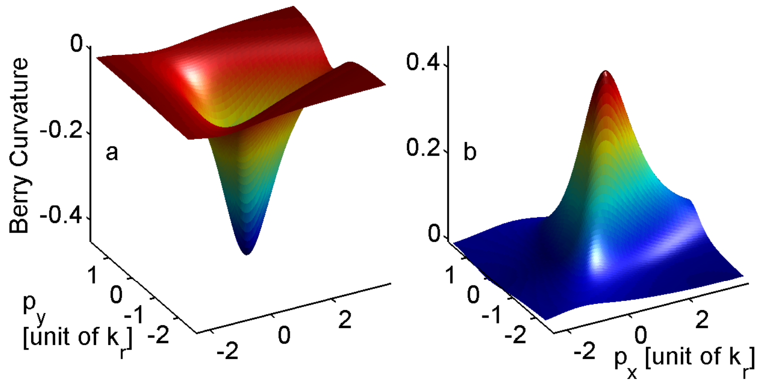


FIG. S4: **Berry curvature in the momentum space for case II**. (a) and (b) show the lowest and the second bands, respectively. $\theta = \pi/4$. The other experimental parameters are the same as Fig. 2 in the main text. For case I, the Berry curvature is a delta function at the Dirac point.
